# Supplementary material for: Neutrinos from Stored Muons (nuSTORM)
Source: arXiv:2505.06137 source file (2025-05-14)
Supplement: Supplementary file 1 [file 10-Appendix.tex]

\appendix

\section*{\Large Appendix}

\graphicspath{ {10-Appendix/10-01-Simulation/Figures/} }

\section{Simulation}
\label{Appen:Simulation}
The studies are based on preliminary simulations to estimate the
fluxes of neutrinos which might be expected at the front face of a
detector of volume 5\,m x 5\,m x 5\,m placed 50\,m downstream of the end
of the nuSTORM production straight.
This is purpose written code which tracks charged particles from the
production target, down the transfer line  into the production
straight and for multiple turns round the nuSTORM ring.
These particles are assumed to propagate down the optical axis of the
machine and with uniform bending fields and without fringe fields.
The pions decay with the correct distribution of lifetimes and produce
muons and neutrinos with the correct kinematic distributions.
The muons are likewise allowed to decay with the correct lifetime and
the decay products are given the correct kinematic distributions.
The resulting neutrinos are tracked and the position and momentum of
those which cross the plane of the front face of the detector and are
within 10\,m of the detector centre are recorded.
Those within $\pm 2.5\,\text{m}$ in the vertical and horizontal plane
are counted as the flux crossing the front face of the detector. 

In order to improve the accuracy of the simulation, the distributions are
smeared using the results of two other programmes.
The momentum distribution and emittance of the pion beam which leaves
the production region are modelled using FLUKA and these distributions
define the starting conditions of the beam.
The magnetic lattice of the transfer line and production straight are
modelled using BDSIM.
These numbers are used to model the emittance of the beam as it
travels through the transfer line, down the production straight and is
finally captured by the ring. The acceptance of the nuSTORM ring to muons is modelled using the results from %the paper Racetrack FFAG muon decay ring 
\cite{Lagrange:2018rt}. This is used to smear the position and momentum of the decay products from both the pion decay and the subsequent muon decay.

\section{Background estimates}
\label{Appen:BkgEstimates}

We have modelled the number of neutrinos we expect from the pion flash in the production straight and the background
from muons which decay before they reach the first bend. We have also modelled the number of neutrinos produced by
muons which are captured in the nuSTORM ring and subsequently decay. There are possible additional backgrounds to these two
sources; we have investigated those and have ignored any background which is less than 1\% of the signal. A summary of
the calculations and reasoning is given below.

\subsection{Decays in the transfer line at $E_{\pi}$=5 GeV}
Neutrinos from pion decay in the transfer line which reach the detector will overlap in time from the decays in the 
production straight. Figure \ref{fig:E5TLPi} shows the x and y distributions of neutrinos from pion decay in the transfer line at the plane of the detector front face. If we look at the y position (vertical) of the neutrinos which reach the plane, we see that the 
distribution is symmetrical and strongly peaked around zero. The x position has a similar shape, but the transfer line is at an angle
to the production straight and so only the tail of the distribution passes through the detector front  face.  Only 11 neutrinos from 
500k pions at the target arrive at the detector,  compared with the pion flash in the production straight where  7138 neutrinos 
reach the detector from 50k pions; a contamination of less than 0.01\%. The mean energy of these neutrinos is 0.06 GeV; 
in order to  be thrown wide enough by the Q value from the decay to reach the detector, the neutrino must have a low energy 
in the nuSTORM rest frame. This source can therefore be ignored. Of the  81835  muons produced by pion decay 195 decay before the 
end of the transfer line and even if all the neutrinos produced by the muon decay reach  the detector, then this represents 
only 0.27\% of the flash signal. Although some of the muons will make it from the transfer line into the production straight,
most of them will be absorbed by the material surrounding the beam tunnel, or by the material inside the tunnel. They
will be brought to rest by about 15~m of soil. These muons will decay at rest and the resulting neutrinos will be distributed 
isotropically. The acceptance of a detector with a $25~\text{m}^2$ front face at a distance of around 250~m means results in only 8 of these neutrinos being visible in the detector, 
and those at very low energy. We conclude that neutrinos from muon decay in the transfer line can also be ignored.

\subsection{Decays in the transfer line at $E_{\pi}$=3 GeV}

At 3 GeV the distribution is wider, as can be seen in Figure \ref{fig:E3TLPi}. The peak at zero is lower in the y position but the tail is higher in the x position.
The combined effect of these is that 34 neutrinos arrive at the detector and their mean energy is slightly higher (0.10 GeV),
because the forward beaming from the pion momentum is smaller and thus the Q value can push the resulting
neutrinos out to wider angles. The contribution at less than 0.03\% is still negligible.
The muon decays in the production straight are still at a low level and even if the transfer line was directed straight at the detector they would still only produce  a rate of around 0.2\%.

The same argument on the muons which are bought to rest by the surrounding material, but in a shorter distance, applies for the 3 GeV sample.

Hence, decays in the transfer line for both pions and muons at pion energies of 3 and 5 GeV are at a level we ignore in this 
study.

\begin{figure}
  \centerline{
  \includegraphics[scale=0.45]{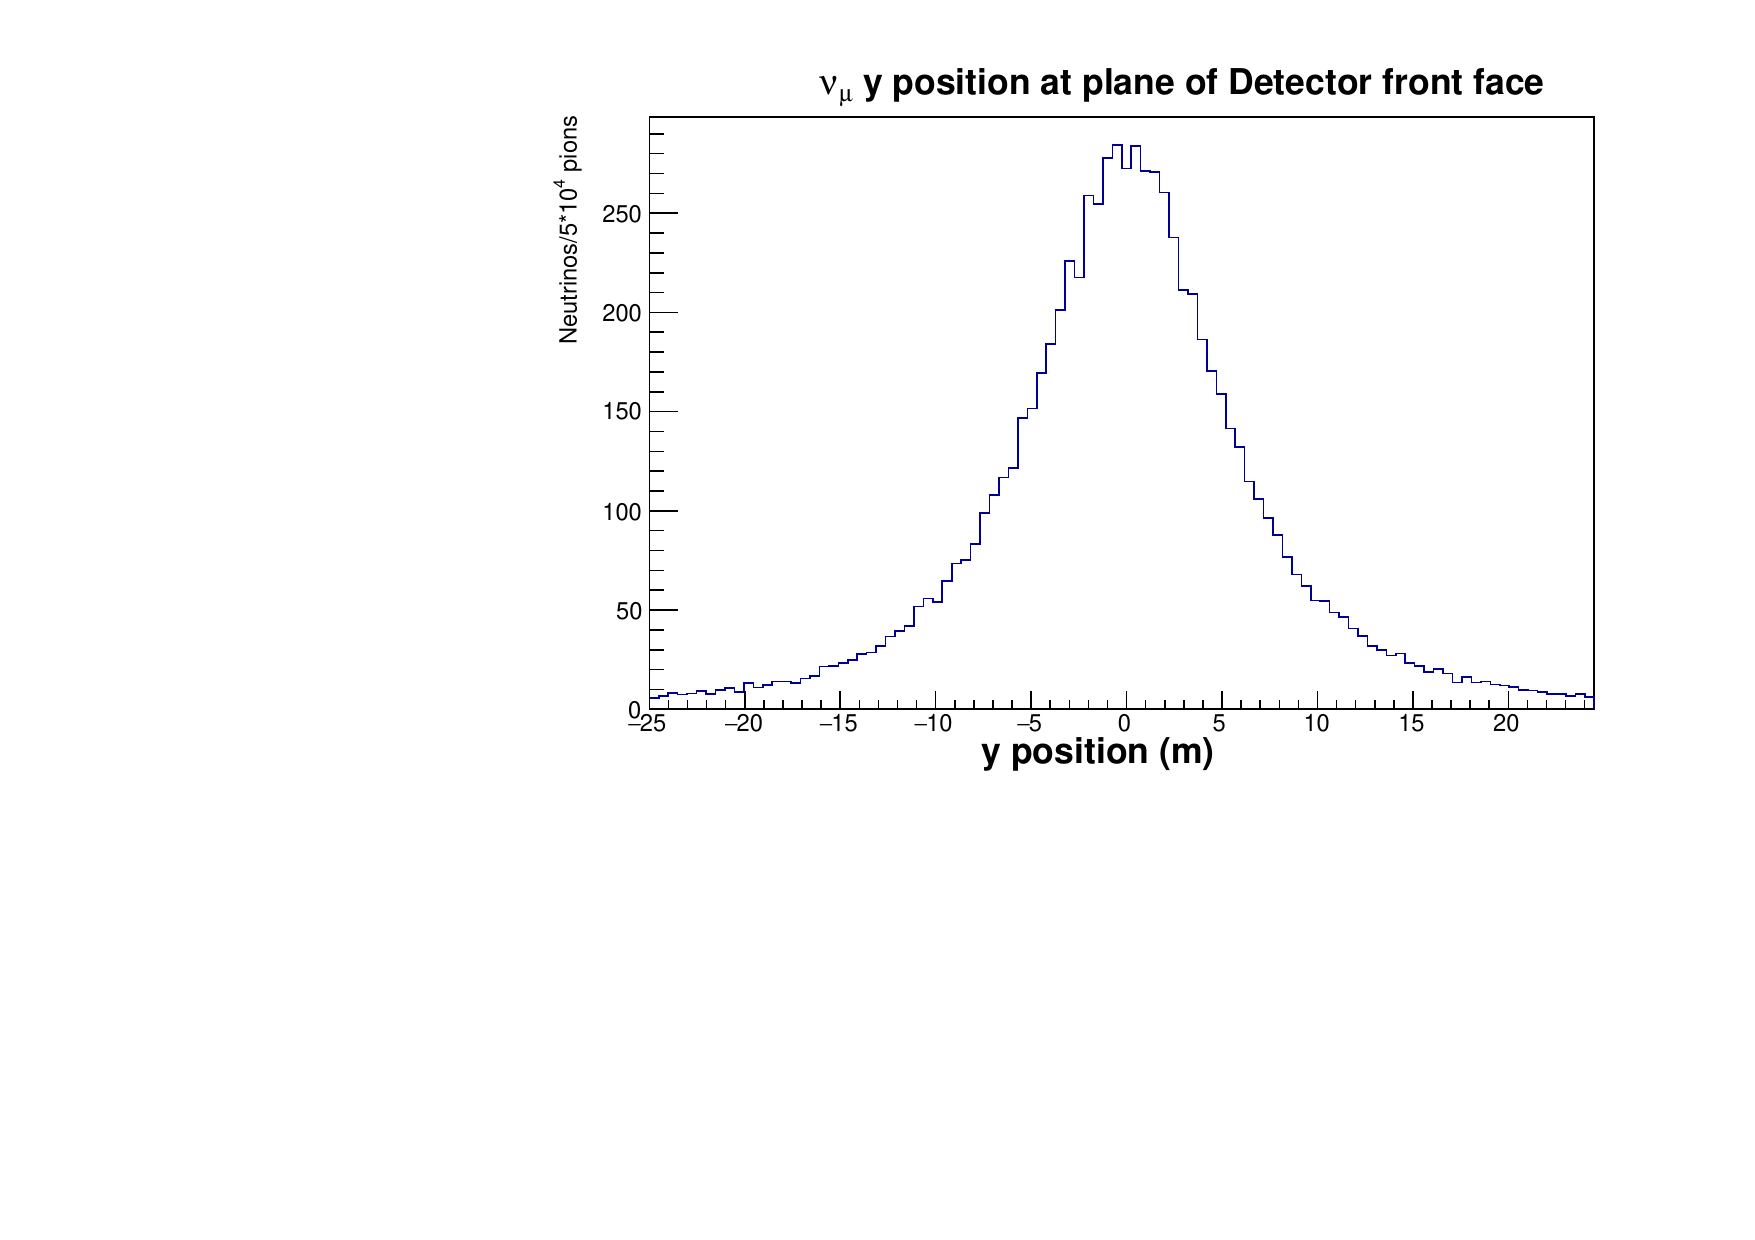}
  \includegraphics[scale=0.45]{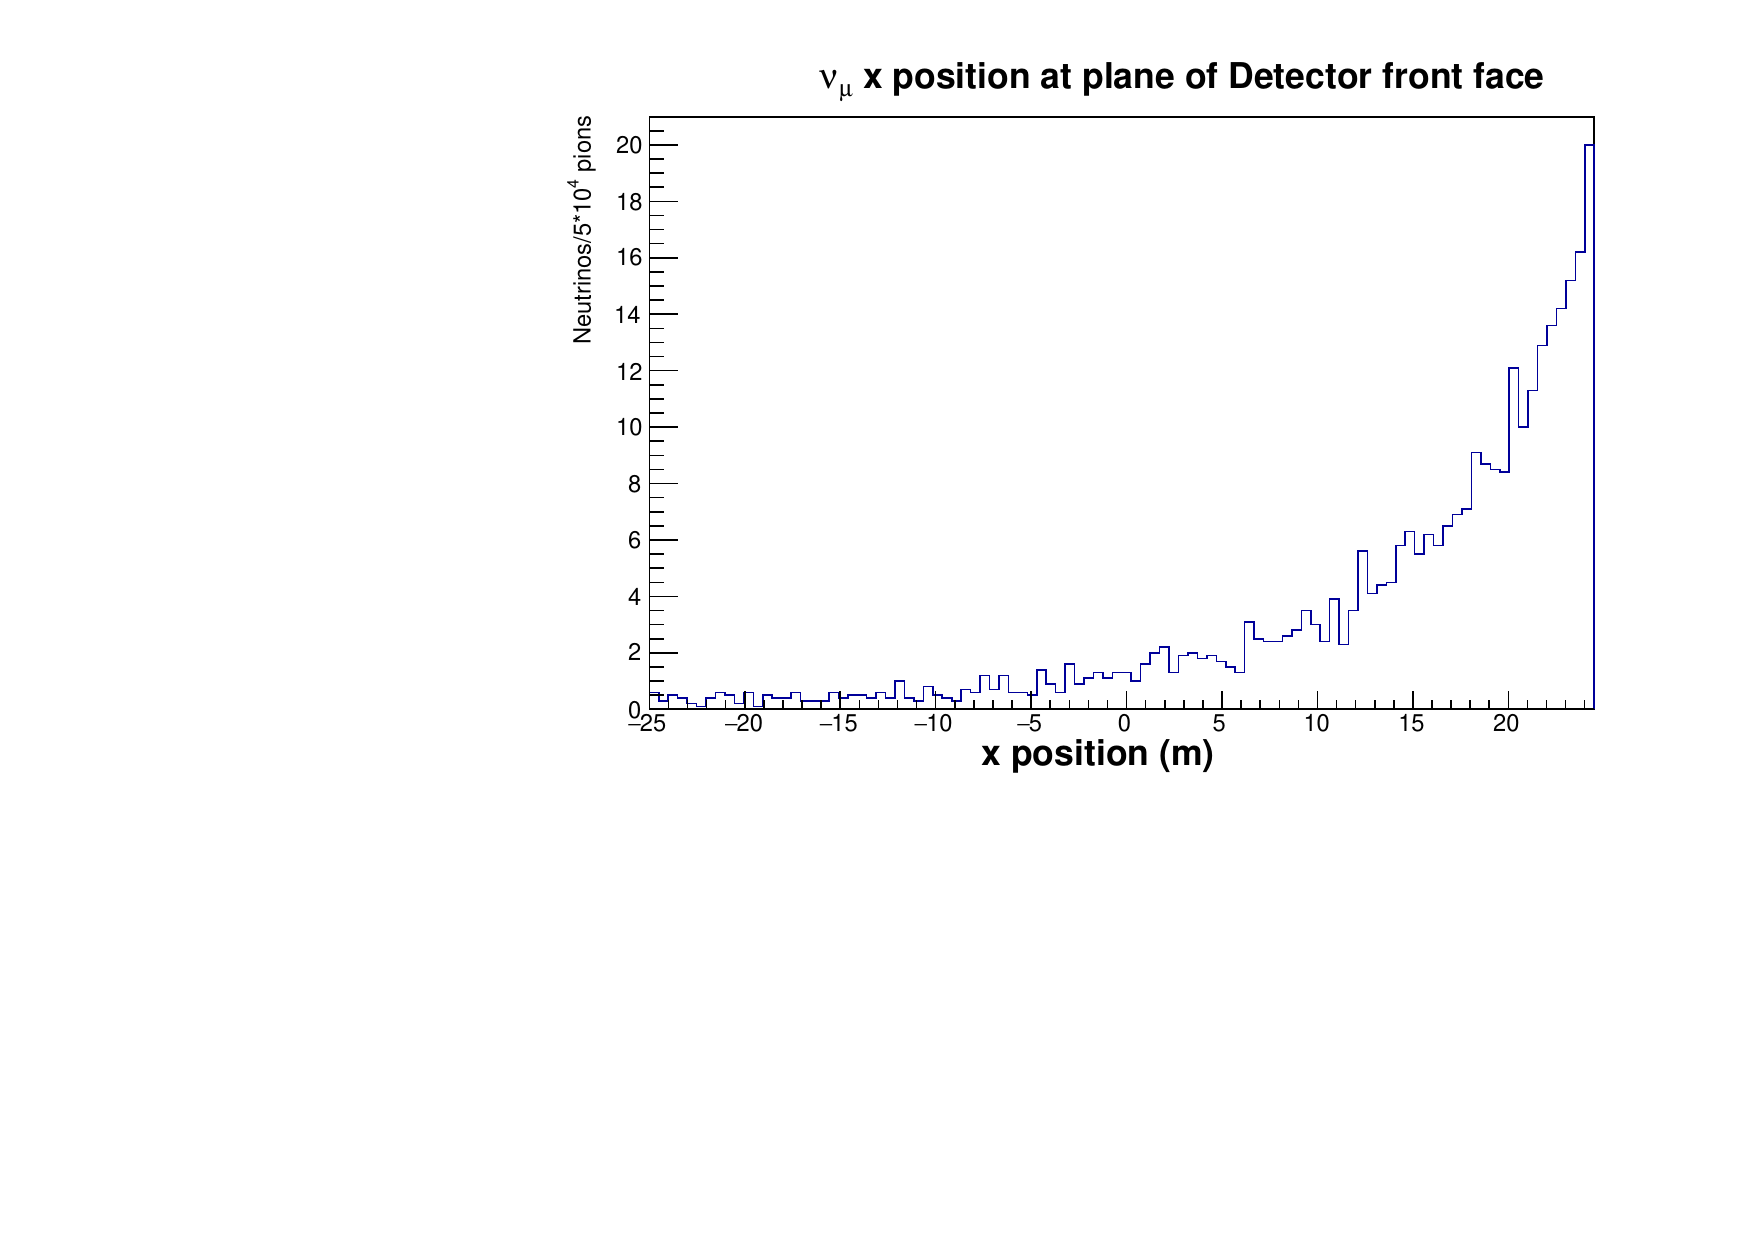}
  }
  \caption{Neutrinos from pion decay in the transfer line at the plane defined by the front face of the detector. Y distribution (left), X distribution (right)}
  \label{fig:E5TLPi}
\end{figure}

\begin{figure}
  \centerline{
  \includegraphics[scale=0.45]{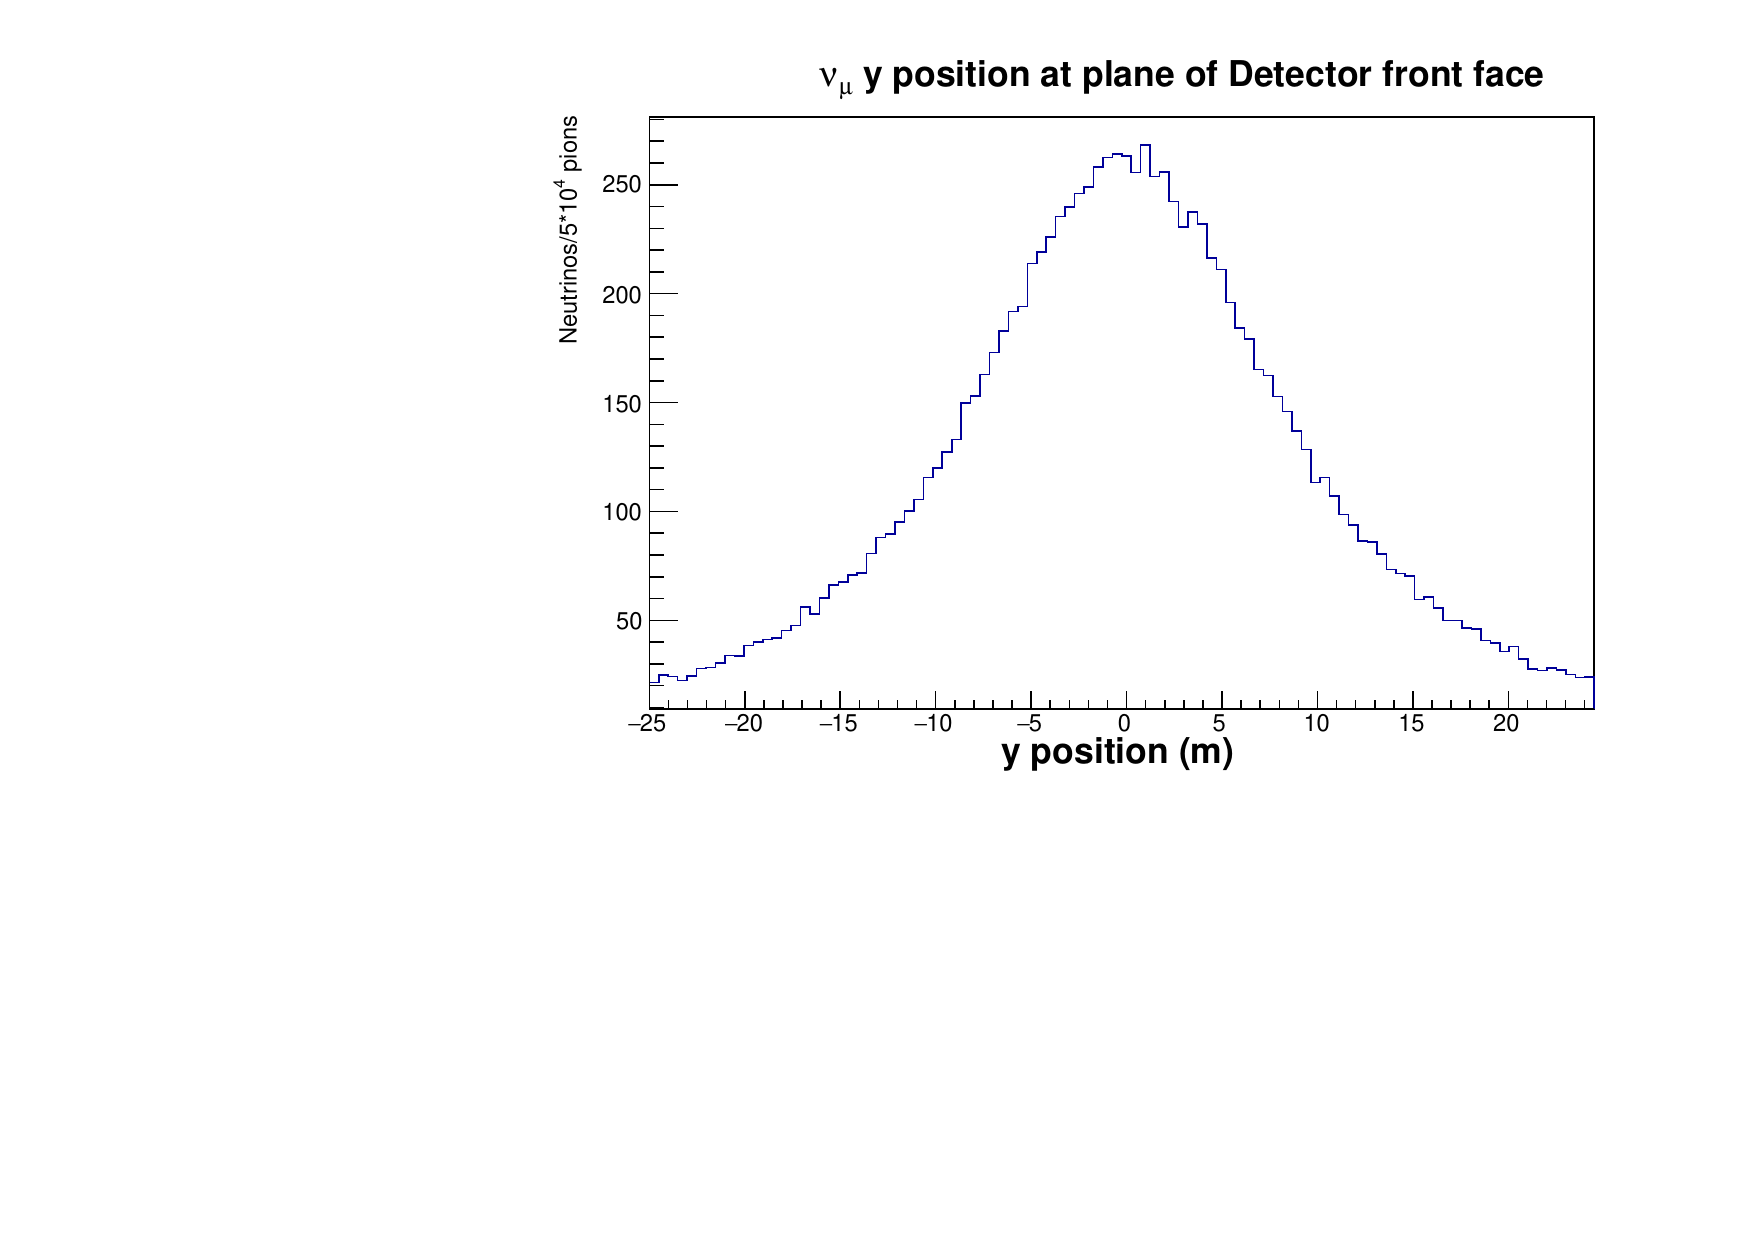}
  \includegraphics[scale=0.45]{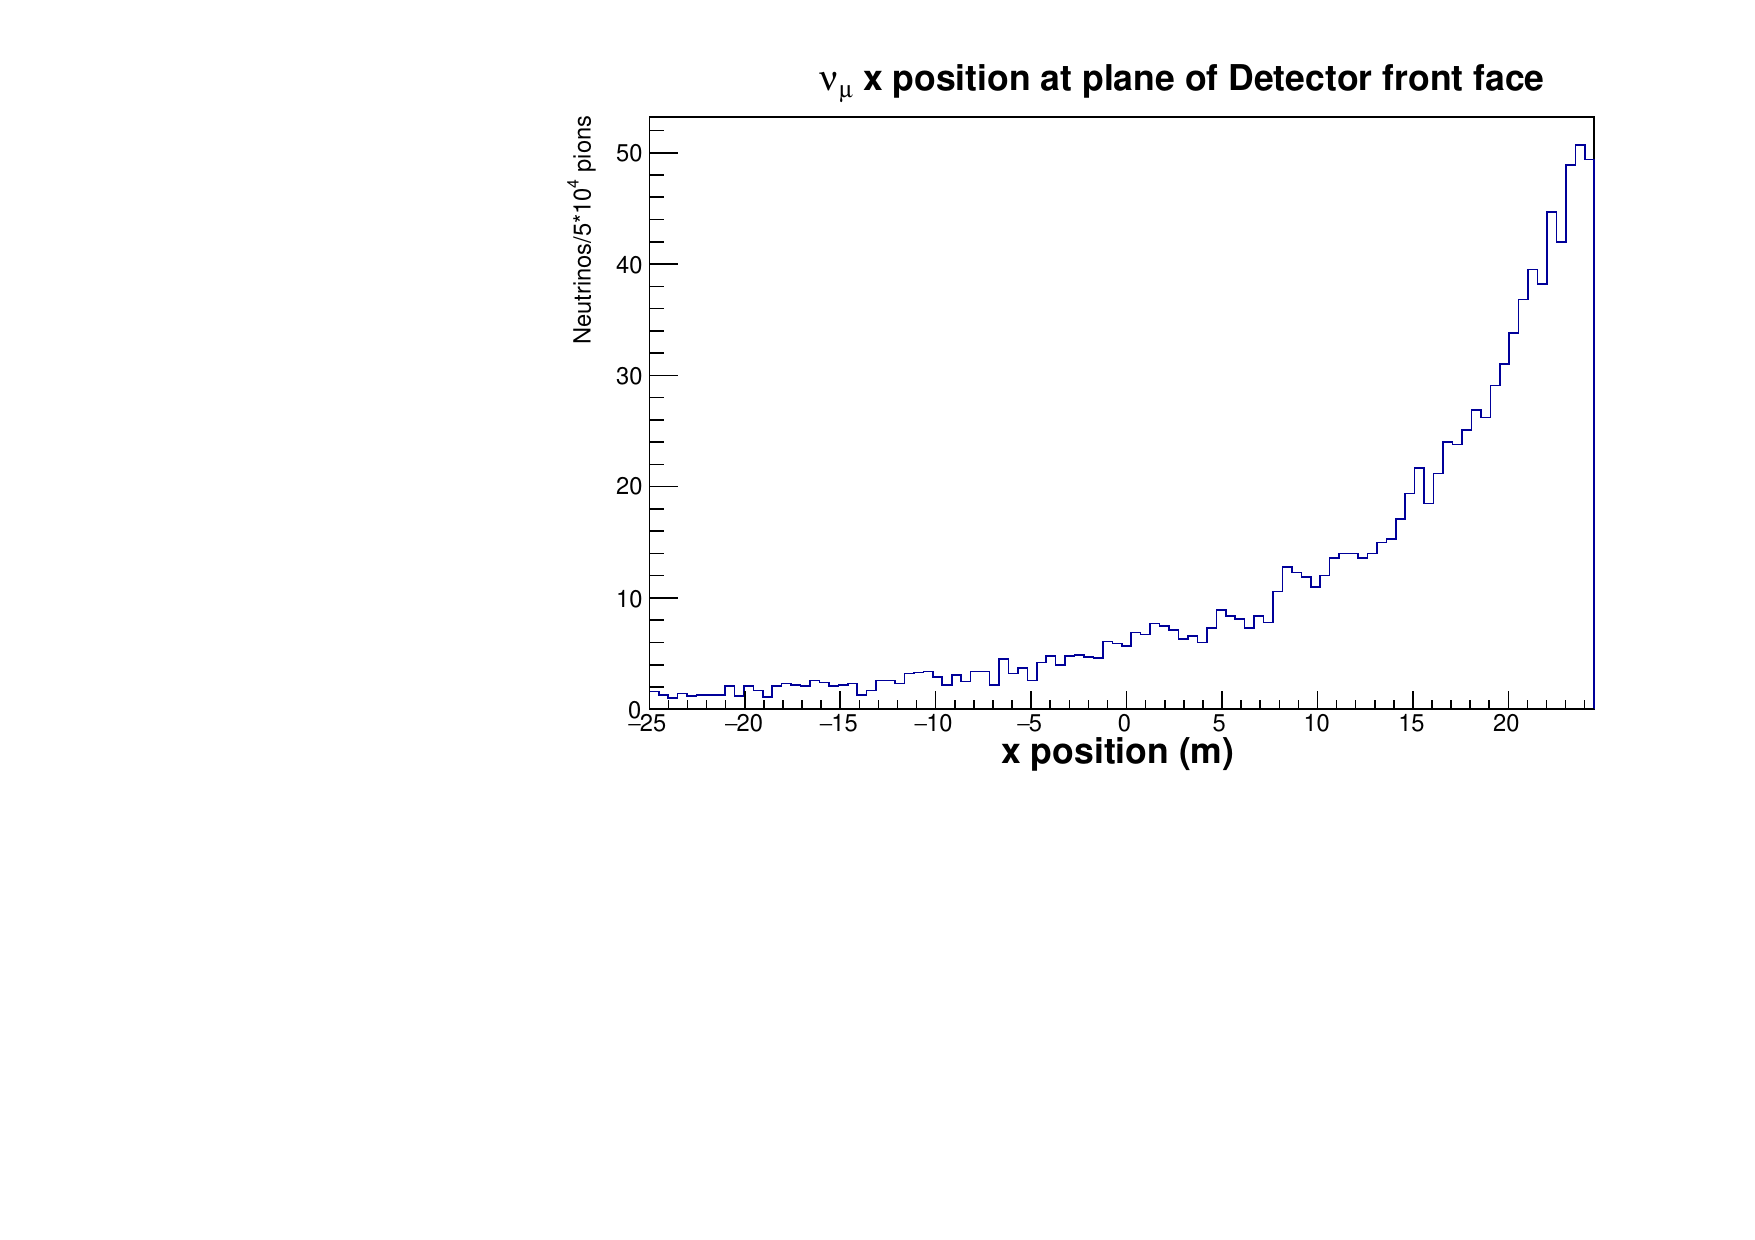}
  }
  \caption{Neutrinos from pion decay in the transfer line at the plane defined by the front face of the detector. Y distribution (left), X distribution (right)}
  \label{fig:E3TLPi}
\end{figure}

\subsection{Decays at the start of the first bend}
We don't have a design which accurately models what happens to the pions as they enter the first bend at the
end of the production straight. However we know from modelling of the transfer line that by the time the
beam has been bent by 8 degrees neutrinos produced by the beam have only a small chance of reaching the
detector. If we look at the number of pions which decay in the the arc as the beam turns through 8 degrees and assume
that the acceptance for these neutrinos is the average of that for a beam at zero degrees and a beam at 8 degrees,
then the background is about 1\%. And since most pions will actually hit an absorber and at worst decay at
rest, the actual background will be smaller and at much lower energies. 

\subsection{Kaons in the transfer line}
We have not modelled Kaon kinematics, but the number produced at the target is significantly lower than the number of pions. 
Even if all of those decay, the number of Kaon decays is less than the number of pion decays and there is no reason to
believe  the acceptance for their neutrinos will be any greater than those from pion decays. We conclude the number
of kaon neutrinos is much less than our 1\% cutoff for modelling.
